# Supplementary material for: Non-Hermitian phase-biased Josephson junctions
Source: arXiv:2307.15472 source file (2024-11-12)
Supplement: Supplementary file 1 [file NHJJ_SM_V6.pdf]

# Supplemental Material for "Non-Hermitian phase-biased Josephson junctions"

Jorge Cayao[1] and Masatoshi Sato[2]
[1]*Department of Physics and Astronomy, Uppsala University, Box 516, S-751 20 Uppsala, Sweden*
[2]*Yukawa Institute for Theoretical Physics, Kyoto University, Kyoto 606-8502, Japan*
(Dated: October 11, 2024)

In this supplemental material we discuss the derivation of the effective Hamiltonian used in the main text to study non-Hermitian Josephson junctions and provide further analysis of their symmetries and non-Hermitian topology. We also discuss the Andreev bound states found in our models in the Hermitian regime and give analytical expressions for the supercurrents of the effective non-Hermitian models. Furthermore, we present the derivation of the supercurrent formula given by Eq. (2) of the main text and extend the discussion on the supercurrent enhancement.

## S1. DERIVATION OF THE EFFECTIVE HAMILTONIAN

In the main text, we describe Josephson junctions (JJs) coupled to leads by an effective non-Hermitian Hamiltonian $H_{\rm eff}$. In this section, we derive the effective Hamiltonian in an exact manner. For this purpose, we consider a JJ and leads described by the Hamiltonians $H_{\rm JJ}$ and $H_{\rm L}$, respectively. The total Hamiltonian is

$$H = \begin{pmatrix} H_{\rm L} & T \\ T^{\dagger} & H_{\rm JJ} \end{pmatrix}\,, \tag{S1}$$

where $T$ is the hopping matrix between the JJ and the lead L. We assume that the lead is semi-infinite so we can treat it as an environment. From the retarded Green's function of the total system, we below derive the Green's function of the JJ under the influence of the lead, which gives the effective Hamiltonian.

From the equation of motion, we can show that the total retarded Green's function obeys the equation

$$(\omega - H)G^{r}(\omega) = 1, \tag{S2}$$

where we have omitted the infinite small imaginary part of $\omega + i\eta$ for simplicity. This equation is equivalent to

$$\begin{pmatrix} \omega - H_{\rm L} & -T \\ -T^{\dagger} & \omega - H_{\rm JJ} \end{pmatrix} \begin{pmatrix} G^{r}_{\rm L} & G^{r}_{\rm LJJ} \\ G^{r}_{\rm JJL} & G^{r}_{\rm JJ} \end{pmatrix} = \begin{pmatrix} 1 & 0 \\ 0 & 1 \end{pmatrix}\,, \tag{S3}$$

with $G^{r}_{\rm L(JJ)}$ the Green's function of the lead (JJ) and $G^{r}_{\rm LJJ/JJL}$ the Green's function between the lead and the JJ. In terms of the components, we have

$$\begin{aligned} (\omega - H_{\rm L})G^{r}_{\rm L} - TG^{r}_{\rm JJL} &= 1\,, \\ (\omega - H_{\rm L})G^{r}_{\rm LJJ} - TG^{r}_{\rm JJ} &= 0\,, \\ -T^{\dagger}G^{r}_{\rm L} + (\omega - H_{\rm JJ})G^{r}_{\rm JJL} &= 0\,, \\ -T^{\dagger}G^{r}_{\rm LJJ} + (\omega - H_{\rm JJ})G^{r}_{\rm JJ} &= 1\,. \end{aligned} \tag{S4}$$

Then, the second equation leads to

$$G^{r}_{\rm LJJ} = (\omega - H_{\rm L})^{-1}TG^{r}_{\rm JJ} = g_{\rm L}(\omega)TG^{r}_{\rm JJ}\,, \tag{S5}$$

where

$$g^{r}_{\rm L}(\omega) = (\omega - H_{\rm L})^{-1} \tag{S6}$$

is the Green's function of the isolated semi-infinite lead. Substituting Eq. (S5) into the last expression of Eqs. (S4), we obtain the Green's function of the JJ under the influence of the semi-infinite lead,

$$G^{r}_{\rm JJ} = [(\omega - H_{\rm JJ}) - T^{\dagger}g_{\rm L}(\omega)T]^{-1}\,, \tag{S7}$$

which defines the effective Hamiltonian of the JJ as

$$G^{r}_{\rm JJ} = [\omega - H_{\rm eff}]^{-1}\,. \tag{S8}$$

Thus, the effective Hamiltonian reads

$$H_{\text{eff}} = H_{\text{JJ}} + \Sigma^r(\omega)\,, \tag{S9}$$

with the self-energy

$$\Sigma^r(\omega) = T^\dagger g^r_{\text{L}}(\omega) T\,. \tag{S10}$$

Therefore, the effective Hamiltonian given by Eq. (S9) incorporates the effects of the lead in an exact manner.

### S1.1. Self-energy

Having established that the incorporation of the leads is exact, we now discuss how to evaluate the self-energy. The main text discusses two types of systems: a system with coupled normal leads and a system coupled to a ferromagnet lead. Without loss of generality, we derive below the self-energy by the semi-infinite ferromagnet lead; a similar analysis leads to the self-energy by a semi-infinite normal lead.

As explained in the previous section, the evaluation of the self-energy requires the retarded Green's function of the isolated semi-infinite lead $g^r_{\text{L}}(\omega)$. Using the recursive Green's function approach, one can calculate the isolated semi-infinite lead's Green's function at the boundary. The Green's function at the boundary is diagonal in the Nambu space, with the electron (e) and hole (h) parts given by [1, 2]

$$g^{e(h)}_{\sigma\sigma}(\omega) = \begin{cases} \dfrac{1}{|t_{\text{L}}|}\left[\dfrac{\omega-\epsilon^{e(h)}_\sigma}{2|t_{\text{L}}|} - \text{sgn}(\omega-\epsilon^{e(h)}_\sigma)\sqrt{\left(\dfrac{\omega-\epsilon^{e(h)}_\sigma}{2|t_{\text{L}}|}\right)^2 - 1}\,\right]\,, & |(\omega-\epsilon^{e(h)}_\sigma)/2|t_{\text{L}}|| > 1 \\ \dfrac{1}{|t_{\text{L}}|}\left[\dfrac{\omega-\epsilon^{e(h)}_\sigma}{2|t_{\text{L}}|} - i\sqrt{1-\left(\dfrac{\omega-\epsilon^{e(h)}_\sigma}{2|t_{\text{L}}|}\right)^2}\,\right]\,, & |(\omega-\epsilon^{e(h)}_\sigma)/2|t_{\text{L}}|| < 1\,, \end{cases} \tag{S11}$$

with $\sigma =\uparrow,\downarrow$, $\epsilon^e_\uparrow = -\epsilon^h_\uparrow = 2t_{\text{L}} - \mu_{\text{L}} + B$, and $\epsilon^e_\downarrow = -\epsilon^h_\downarrow = 2t_{\text{L}} - \mu_{\text{L}} - B$, where $t_{\text{L}}$ and $\mu_{\text{L}}$ are the next nearest neighbor hopping and the chemical potential in the lead, respectively, and $B$ is the Zeeman field due to ferromagnetism. Equation (S11) produces the imaginary part via the local density of states (LDOS) $\rho_{\text{L}} = -(1/\pi)\text{Im}g^r_{\text{L}}$:

$$[\rho_{\text{L}}(\omega)]^{\text{e(h)}}_\sigma = \frac{\theta(2|t_{\text{L}}| - |\omega-\epsilon^{e(h)}_\sigma|)}{|t_{\text{L}}|\pi}\sqrt{1-\left(\frac{\omega-\epsilon^{e(h)}_\sigma}{2|t_{\text{L}}|}\right)^2}\,, \tag{S12}$$

which is nonzero within the bandwidth $|(\omega-\epsilon^{e(h)}_\sigma)/2|t_z|| < 1$.

Using the above result, we evaluate the self-energy $\Sigma^r = T^\dagger g^r_{\text{L}} T$. Since $T$ is finite between the nearest neighbor sites between the lead and the JJ, the self-energy is nonzero only at sites attached to the lead,

$$\Sigma^{e(h)}_{1_{\text{S}}1_{\text{S}}}(\omega) = \langle 1_{\text{S}}|\,T^\dagger\,|1_{\text{L}}\rangle\,\langle 1_{\text{L}}|\,g^{e(h)}(\omega)\,|1_{\text{L}}\rangle\,\langle 1_{\text{L}}|\,T\,|1_{\text{S}}\rangle\,, \tag{S13}$$

where $1_{\text{L}}$ and $1_{\text{S}}$ are the adjacent sites on the lead and the JJ, respectively. In terms of the hopping amplitude $\bar{\tau}$ between the lead and the JJ, we have $\langle 1_{\text{L}}|\,T\,|1_{\text{S}}\rangle = -\bar{\tau}\sigma_0$, and thus the self-energy reads

$$\Sigma^{e(h)}_{1_{\text{S}}1_{\text{S}}} = \begin{pmatrix} |\bar{\tau}|^2 g^{e(h)}_{\uparrow\uparrow} & 0 \\ 0 & |\bar{\tau}|^2 g^{e(h)}_{\downarrow\downarrow} \end{pmatrix}, \tag{S14}$$

with $g^{e(h)}_{\uparrow\uparrow}$ and $g^{e(h)}_{\downarrow\downarrow}$ in Eqs. (S11). Whereas the self-energy term contains both the real and imaginary parts, only the imaginary part gives non-Hermitian effects. The real part only shifts the diagonal entries in $H_{\text{JJ}}$.

To further explore the impact of the non-Hermitian component, we employ the wide-band approximation $|(\omega - \epsilon^{e(h)}_\sigma)/(2t_{\text{L}})| \ll 1$, commonly used in quantum transport [3]. This approximation enables to neglect of the $\omega$-dependence in the Green's function of the lead but still considers $B$ and $\mu_{\text{L}}$ to be large enough to induce different imaginary terms in $g^{e(h)}_{\sigma\sigma}$ for different spins. Now (the imaginary part of) the self-energy reads

$$\Sigma^r(\omega) \approx \begin{pmatrix} \Sigma^{\text{e}}(\omega=0) & 0 \\ 0 & \Sigma^{\text{h}}(\omega=0) \end{pmatrix}, \tag{S15}$$

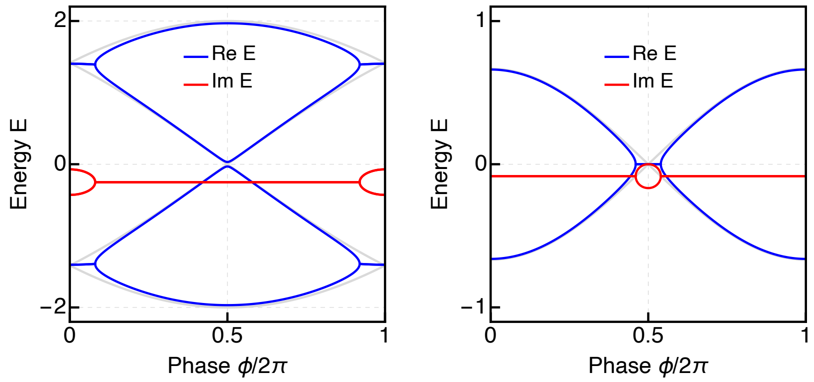


FIG. S1. Left: Re (blue) and Im (red) parts of the eigenvalues given by Eq.(4) of the main text as a function of $\phi$ at $\Gamma_L = 0.5$, $\Gamma_R = 0$. Right: Re (blue) and Im (red) parts of the eigenvalues given by Eq.(6) of the main text as a function of $\phi$ at $\Gamma_\uparrow = 0.5$, $\Gamma_\downarrow = 0$. In both panels, the gray curves correspond to the Hermitian regime. Parameters: $\Delta = 1$, $t = 1$, $\varepsilon_\alpha = 0$.

where

$$\Sigma^{\mathrm{e,h}}(\omega = 0) = -i\Gamma\sigma_0 - i\gamma\sigma_z\,, \tag{S16}$$

with $\Gamma = (\Gamma_\uparrow + \Gamma_\downarrow)/2$ and $\gamma = (\Gamma_\uparrow - \Gamma_\downarrow)/2$. Here, $\Gamma_\sigma = \pi|\bar{\tau}|^2\rho_{\mathrm{L}}^\sigma$, where $\rho_{\mathrm{L}}^\sigma$ is the spin-polarized surface density of states of the lead,

$$\rho_{\mathrm{L}}^{\uparrow(\downarrow)} = \frac{1}{t_z\pi}\sqrt{1 - \left[\frac{\mu_{\mathrm{L}} \mp B}{(2t_z)}\right]^2}\,. \tag{S17}$$

Thus, $\Gamma_\sigma$ is controllable by $B$, $\mu_{\mathrm{L}}$, $t_z$, and $\bar{\tau}$. The self-energy in Eq. S15 has negative imaginary parts corresponding to decay rates. With the obtained self-energy, the effective Hamiltonian $H_{\mathrm{eff}}$ in Eq. (S9) describes the JJ coupled to a ferromagnet lead studied in the main text. Similarly, we can obtain the self-energy for a junction coupled to a normal lead, as in the case of the first model discussed in the main text, just by setting $B = 0$ in the above result. The effective Hamiltonian with a zero-frequency self-energy is used in the main text [Eq. (1)] to explore non-Hermitian JJs.

### S1.2. Weak, intermediate, or strong coupling regime

Using the result in the previous section, we compare here the hopping $\bar{\tau}$ between the lead and the JJ with the superconducting pair potential $\Delta$. Depending on the ratio of these energy scales, superconducting heterostructures have three regimes, weak ($\bar{\tau} \ll \Delta$), intermediate ($\bar{\tau} \sim \Delta$), and strong coupling ($\bar{\tau} \gg \Delta$) regions [4].

Here, we should note that $\bar{\tau}$ can be much smaller than $\Gamma_\sigma$: From Eq. (S16), we have

$$\bar{\tau} = \sqrt{\frac{\Gamma_\sigma}{\pi\rho_{\mathrm{L}}^\sigma}}\,. \tag{S18}$$

Thus, for the case of $\rho_{\mathrm{L}}^\sigma = 1$ and $\Gamma_\sigma = 1$, we estimate $\bar{\tau} = 0.56$. Therefore, even when $\Gamma_\sigma$ is comparable with $\Delta = 1$, as in our models in the main text, we may realize the weak coupling regime $\Delta = 1 > \bar{\tau} = 0.56$.

A smaller $\Gamma_\sigma$ easily realizes the weak coupling regime. In Fig. S1, we show the phase-dependent Andreev spectra of the first two models in the main text with a smaller $\Gamma_\sigma$. The spectra clearly indicate exceptional points (EPs), and our conclusion holds even for smaller $\Gamma_\sigma$.

## S2. SYMMETRIES AND NON-HERMITIAN TOPOLOGY OF JOSEPHSON JUNCTIONS

### S2.1. Particle-hole symmetry in the effective Hamiltonian of Josephson Junctions

Here, we discuss particle-hole symmetry (PHS) in the effective Hamiltonian of Josephson Junctions. PHS is a proper symmetry in superconductors, which is defined by

$$\hat{C}\psi_{\alpha i}^{\dagger}\hat{C}^{-1}=\sum_{j}\psi_{\alpha j}(U_C^{\alpha})^{*}_{ji}\,,\quad \hat{C}\psi_{\alpha i}\hat{C}^{-1}=\sum_{j}\psi_{\alpha j}^{\dagger}(U_C^{\alpha})_{ji}\,, \tag{S19}$$

where $\psi_{\alpha i}$ represents the Nambu spinor, $\alpha$ is the label distinguishing the JJ ($\alpha=1$) and the lead ($\alpha=2$), $i$ represents the degrees of freedom such as the coordinate and spin, and $U_C^{\alpha}$ is a unitary matrix. Since PHS is a local symmetry, it does not mix different $\alpha$. For the quadratic Hamiltonian

$$\hat{H}=\sum_{\alpha i,\beta j}\psi_{\alpha i}^{\dagger}(H)_{\alpha i,\beta j}\psi_{\beta j}\,, \tag{S20}$$

the above operations reproduce the standard form of PHS:

$$[\hat{H},\hat{C}]=0\quad\Leftrightarrow\quad (U_C^{\alpha})_{ip}(H^T)_{\alpha p,\beta q}(U_C^{\beta\dagger})_{qj}=-(H)_{\alpha i,\beta j}\,. \tag{S21}$$

To examine particle-hole symmetry in the effective Hamiltonian, let us consider the retarded Green function of the JJ

$$(G_{\mathrm{JJ}}^{\mathrm{r}})_{ij}=-i\theta(t)\langle\psi_{1i}(t)\psi_{1j}^{\dagger}+\psi_{1j}^{\dagger}\psi_{1i}(t)\rangle, \tag{S22}$$

where $\psi_{1i}$ is the Nambu spinor in the JJ. Then, particle-hole symmetry $\hat{C}^{-1}\hat{H}\hat{C}=\hat{H}$ leads to

$$\begin{aligned}
\langle\psi_{1i}(t)\psi_{1j}^{\dagger}\rangle &= \mathrm{tr}(e^{-\beta\hat{C}^{-1}\hat{H}\hat{C}}e^{i\hat{C}^{-1}\hat{H}\hat{C}t}\psi_{1i}e^{-i\hat{C}^{-1}\hat{H}\hat{C}t}\psi_{1j}^{\dagger})/\mathrm{tr}(e^{\beta\hat{H}})\\
&= \mathrm{tr}(e^{-\beta\hat{H}}e^{i\hat{H}t}\hat{C}\psi_{1i}\hat{C}^{-1}e^{-i\hat{H}t}\hat{C}\psi_{1j}^{\dagger}\hat{C}^{-1})/\mathrm{tr}(e^{\beta\hat{H}})\\
&= \left[\sum_{kl}\mathrm{tr}(e^{-\beta\hat{H}}e^{i\hat{H}t}\psi_{1k}^{\dagger}e^{-i\hat{H}t}\psi_{1l})(U_C^1)_{ki}(U_C^1)^{*}_{lj}\right]/\mathrm{tr}(e^{\beta\hat{H}})\\
&= \left[\sum_{kl}(\mathrm{tr}(\psi_{1l}^{\dagger}e^{i\hat{H}t}\psi_{1k}e^{-i\hat{H}t}e^{-\beta\hat{H}}))^{*}(U_C^1)_{ki}(U_C^1)^{*}_{lj}\right]/\mathrm{tr}(e^{\beta\hat{H}})\\
&= \sum_{kl}(U_C^1)^{\dagger}_{jl}\langle\psi_{1l}^{\dagger}\psi_{1k}(t)\rangle^{*}(U_C^1)_{ki}\,,
\end{aligned} \tag{S23}$$

where we have used the Hermiticity of $\hat{H}$. Thus, we have

$$\begin{aligned}
(G_{\mathrm{JJ}}^{\mathrm{r}})_{ij} &= (U_C^1)^{\dagger}_{jl}\left[i\theta(t)\langle\psi_{1k}(t)\psi_{1l}^{\dagger}+\psi_{1l}^{\dagger}\psi_{1k}(t)\rangle\right]^{*}(U_C^1)_{ki}\\
&= -(U_C^1)^{\dagger}_{jl}(G_{\mathrm{JJ}}^{\mathrm{r}})^{*}_{kl}(U_C^1)_{ki},
\end{aligned} \tag{S24}$$

which leads to particle-hole symmetry in the effective Hamiltonian for the JJ,

$$(U_C^1)^{T}H_{\mathrm{eff}}^{*}(-\omega,\phi)(U_C^1)^{*}=-H_{\mathrm{eff}}(\omega,\phi). \tag{S25}$$

Here, $\phi$ is the phase difference in the JJ, and we make the $\phi$-dependence in $H_{\mathrm{eff}}$ explicit for later convenience. Note that the PHS in the effective Hamiltonian involves complex conjugation, in contrast to the original PHS in Eq.(S21). Following Ref.[5], we call the complex conjugation version of PHS as PHS$^{\dagger}$. As we show below, PHS$^{\dagger}$ crucially affects the stability of EPs at zero real energy.

### S2.2. Non-Hermitian topology of the model in Fig. 1(a)

First, we examine the model in Fig. 1 (a) of the main text. Here, we consider an $s$-wave gap function and neglect the spin-orbit interactions both in superconductors and leads. Thus, the system supports spin-rotation symmetry.

Using the spin-rotation symmetry, one can show that the reduced Nambu spinor $\psi_{\alpha i}$ with the form

$$\psi_{\alpha i} = \begin{pmatrix} c_{\alpha\uparrow\underline{i}} \\ c^\dagger_{\alpha\downarrow\underline{i}} \end{pmatrix} \equiv \begin{pmatrix} \psi_{\alpha 1\underline{i}} \\ \psi_{\alpha 2\underline{i}} \end{pmatrix} \tag{S26}$$

describes the system, where $\underline{i}$ represents the degrees of freedom other than spin. The Nambu spinor satisfies

$$\hat{S}_{2y}\psi^\dagger_{\alpha 1\underline{i}}\hat{S}^{-1}_{2y} = \hat{S}_{2y}c^\dagger_{\alpha\uparrow\underline{i}}\hat{S}^{-1}_{2y} = -c^\dagger_{\alpha\downarrow\underline{i}} = -\psi_{\alpha 2\underline{i}}, \quad \hat{S}_{2y}\psi^\dagger_{\alpha 2\underline{i}}\hat{S}^{-1}_{2y} = \hat{S}_{2y}c_{\alpha\downarrow\underline{i}}\hat{S}^{-1}_{2y} = c_{\alpha\uparrow\underline{i}} = \psi_{\alpha 1\underline{i}}\,, \tag{S27}$$

where $\hat{S}_{2y}$ is the spin rotation by $\pi$ around the $y$-axis, and thus the system supports PHS in Eq.(S19) with

$$(U^\alpha_C)_{ji} = i(\tau_y)_{\tau'\tau}\delta_{\underline{j},\underline{i}}, \quad (i = (\tau, \underline{i}),\, j = (\tau', \underline{j})). \tag{S28}$$

Consequently, the effective Hamiltonian of the JJ hosts the corresponding PHS$^\dagger$ in Eq.(S25, as shown above. We can also confirm this symmetry directly: The model in Fig. 1(a) of the main text is given by

$$H^{(1)}_{\text{eff}}(\phi) = \begin{pmatrix} \varepsilon_L & \Delta & t & 0 \\ \Delta & -\varepsilon_L & 0 & -t \\ t & 0 & \varepsilon_R & \Delta e^{i\phi} \\ 0 & -t & \Delta e^{-i\phi} & -\varepsilon_R \end{pmatrix} + \begin{pmatrix} -i\Gamma_L & 0 & 0 & 0 \\ 0 & -i\Gamma_L & 0 & 0 \\ 0 & 0 & -i\Gamma_R & 0 \\ 0 & 0 & 0 & -i\Gamma_R \end{pmatrix}, \tag{S29}$$

where $\varepsilon_L$, $\varepsilon_R$, $\Delta$, and $\phi$ are real constants. This model has PHS$^\dagger$ with

$$U_C = \begin{pmatrix} 0 & -1 & 0 & 0 \\ 1 & 0 & 0 & 0 \\ 0 & 0 & 0 & -1 \\ 0 & 0 & 1 & 0 \end{pmatrix}. \tag{S30}$$

Because $U_C$ satisfies $U_C U_C^* = -1$, this symmetry defines class C$^\dagger$ in the symmetry classification in Ref.[5]. This particular type of PHS$^\dagger$ explains why the level crossing at $\phi = \pi$ does not evolve into EPs: According to a general theory in Ref.[6], the point-gap topology intrinsic to non-Hermitian systems ensures the robust existence of EPs. For an EP in the space of $\phi$, the relevant point-gap topological number is 0-dimensional. Moreover, since the level crossing at zero energy is invariant under PHS$^\dagger$, and thus, the point-gap topological number should respect PHS$^\dagger$. However, any class C$^\dagger$ system does not have a 0-dimensional point-gap topological number so the level crossing at zero energy does not evolve into robust EPs.

If we assume $\varepsilon_{\rm L} = \varepsilon_{\rm R}$, as in our calculations in Fig.2, this model also has an accidental parity-time (PT) symmetry,

$$PT\left[H^{(1)}_{\text{eff}}(\phi) + i\frac{\Gamma_L + \Gamma_R}{2}1\right]^* T^\dagger P^\dagger = H^{(1)}_{\text{eff}}(\phi) + i\frac{\Gamma_L + \Gamma_R}{2}1, \tag{S31}$$

where the unitary matrices for time-reversal $T$ and parity $P$ are given by

$$T = \begin{pmatrix} e^{i\phi/2} & 0 & 0 & \\ 0 & e^{-i\phi/2} & 0 & 0 \\ 0 & 0 & e^{i\phi/2} & 0 \\ 0 & 0 & 0 & e^{-i\phi/2} \end{pmatrix}, \quad P = \begin{pmatrix} 0 & 0 & 1 & 0 \\ 0 & 0 & 0 & 1 \\ 1 & 0 & 0 & 0 \\ 0 & 1 & 0 & 0 \end{pmatrix}, \tag{S32}$$

and satisfy $PT(PT)^* = 1$. The PT symmetry enables stable EPs with the energy $E$, which imaginary part is pinned at Im$E = -(\Gamma_L + \Gamma_R)/2$. Note that EPs in Fig. 2(a) have such an imaginary part of the energy. As shown in Ref.[6], the PT-symmetry enables a 0-dimensional $\mathbb{Z}_2$ point-gap topological number, ensuring the stability of EPs in the one-dimensional $\phi$ space. Therefore, the analysis carried out here help understanding the absence and presence of EPs at zero and finite energies, respectively, in the Section "NH JJs with superconductors coupled to different normal leads" of the main text.

### S2.3. Non-Hermitian topology of the model in Fig. 1(b)

In Fig.1 (b) of the main text, we consider a ferromagnetic lead that breaks spin-rotation symmetry. Therefore, the full Nambu spinor

$$\psi_{\alpha i} = \begin{pmatrix} c_{\alpha\uparrow\underline{i}} \\ c_{\alpha\downarrow\underline{i}} \\ c^\dagger_{\alpha\uparrow\underline{i}} \\ c^\dagger_{\alpha\downarrow\underline{i}} \end{pmatrix} \equiv \begin{pmatrix} \psi_{\alpha1\uparrow\underline{i}} \\ \psi_{\alpha1\downarrow\underline{i}} \\ \psi_{\alpha2\uparrow\underline{i}} \\ \psi_{\alpha2\downarrow\underline{i}} \end{pmatrix} \tag{S33}$$

is necessary to describe the system. Since we have the identity

$$\psi^\dagger_{\alpha\tau\sigma\underline{i}} = \sum_{\tau'} \psi_{\alpha\tau'\sigma\underline{i}} (\tau_x)_{\tau'\tau}, \tag{S34}$$

the Hamiltonian should have PHS in Eq.(S19) with $\hat{C} = 1$ and

$$(U^\alpha_C)_{ji} = (\tau_x)_{\tau'\tau} (\sigma_0)_{\sigma'\sigma} \delta_{\underline{j},\underline{i}}, \quad (j = (\tau', \sigma', \underline{j}),\, i = (\tau, \sigma, \underline{i})). \tag{S35}$$

Therefore, the effective Hamiltonian of the JJ obeys PHS$^\dagger$ in Eq.(S25). In the present case, PHS$^\dagger$ defines class D$^\dagger$ in the symmetry classification since $U^\alpha_C$ satisfies $U^\alpha_C (U^\alpha_C)^* = 1$.

In contrast to class C$^\dagger$ in the previous model, class D$^\dagger$ supports a 0-dimensional $\mathbb{Z}_2$ point-gap topological number [6]. Actually, we can confirm that EPs at zero real energy in Fig. 3 (a) and Figs. 4 (a-c) have the non-trivial $\mathbb{Z}_2$ number. Because PHS$^\dagger$ in class D$^\dagger$ is intact under any perturbation in superconductors, these EPs are robust unless the superconducting gap closes or they are pair-annihilated. These EPs are discussed in the section on "NH JJs with a middle N region coupled to a ferromagnet lead" of the main text.

## S3. ANDREEV BOUND STATES IN THE HERMITIAN REGIME

In this section, we compare the Andreev bound states (ABSs) of the models in Eqs. (3), and (5) in the absence of non-Hermiticity with those commonly used in the literature.

### S3.1. Model in Eq. (4) in the Hermitian regime

The eigenvalues for the first model [Eq. (4)] without non-Hermiticity are given by

$$E_j = \pm\sqrt{\delta^2 \pm 2t\Delta\,|\sin(\phi/2)|}\,, \tag{S36}$$

where $\delta = t^2 + \Delta^2$, and $j = 1, 2, 3, 4$ is the index for the different eigenvalues. Thus, in-gap ABSs in the Hermitian regime are given by

$$E_{2,3} = \pm\sqrt{\delta^2 - 2t\Delta\,|\sin(\phi/2)|}\,, \tag{S37}$$

for $t\Delta > 0$. When $|t| = |\Delta|$, the in-gap ABSs show a level crossing at zero energy at $\phi = \pi$, as illustrated in gray curves in Fig.2(a) of the main text.

### S3.2. Model in Eq. (6) in the Hermitian regime

The second model in Eq. (6) hosts in-gap ABSs with the eigenvalues in Eq.(6) in the main text. Without non-Hermiticity, the eigenvalues read

$$E_\pm = \pm\frac{\Delta}{A}\sqrt{C + 2t^4 A\cos(\phi)} \tag{S38}$$

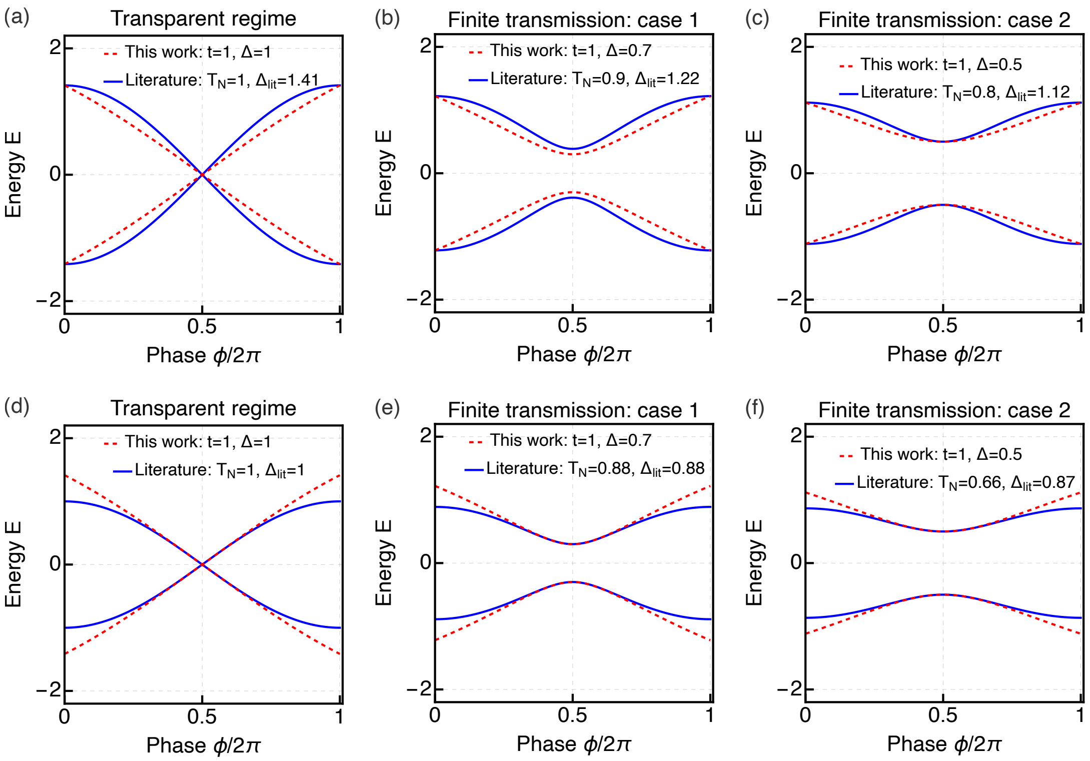


FIG. S2. ABSs as a function of $\phi$ in the Hermitian regime of our first model given by Eq. (S36) (red dashed curves) and using the ABSs from the literature given by Eq. (S40) (blue solid curves). The left, middle, and right columns correspond to distinct parameters, capturing the transparent and finite transmission regimes. (a-c) the ABSs in Eq. (S36) and Eq. (S40) show qualitatively same behaviors. (d-f) The ABSs in Eq. (S36) and Eq. (S40) exhibit exactly the same $\phi$-dependence near $\phi \sim \pi$. Our models, therefore, reproduce the conventional description for ABSs in Hermitian cases.

with $A = 4t^4 + \Delta^4 + 4\Delta^2 t^2$ and $C = 2t^4[4t^4 + (4t^2)\Delta^2 + \Delta^4]$. Since we have $2t^4 A = C$ in the Hermitian case, the eigenvalues are recast into

$$E_\pm = \pm\frac{\Delta\sqrt{C}}{A}\sqrt{1+\cos(\phi)} = \pm\frac{\Delta\sqrt{2C}}{A}\cos(\phi/2)\,. \tag{S39}$$

Thus, they show a level crossing at $\phi = \pi$. In the main text, we illustrate these ABSs in the Hermitian regime in the gray curves of Fig. 3 (a).

### S3.3. Comparison with the standard Hermitian ABSs in the literature

Here, we compare the above ABSs [Eqs. (3) and (5) of the main text] in the Hermitian regime with the standard ABSs in literature. The well-known expressions for the ABSs are commonly derived within the Andreev approximation, where the energy scales are much smaller than the Fermi energy. Here, we focus on the expression for short JJs, as in our models. The standard ABSs in short JJs read [7–9]

$$E_\pm^{\rm lit} = \pm\Delta_{\rm lit}\sqrt{1 - T_{\rm N}\sin^2(\phi/2)}, \tag{S40}$$

where $\Delta_{\rm lit}$ is the superconducting gap, and $T_{\rm N}$ is the normal transmission. For $T_{\rm N} = 1$, it holds $E_\pm^{\rm lit} = \pm\Delta_{\rm lit}\cos(\phi/2)$; thus the ABSs show a level crossing with zero energy at $\phi = \pi$.

*Comparison with model in Eq. (4)*

The ABSs in Eq.(S36) and (S40) show qualitatively the same behavior as functions of $\phi$. See Fig. S2 (a-c). In both cases, they have the maximal (minimal) gap at $\phi = 0$ ($\phi = \pi$). The exact $\phi$-dependence is not the same between

them, but it comes from the difference in the bulk degrees of freedom. Whereas the derivation of Eq. (S40) considers semi-infinite superconductors [7–9], Eq. (S36) considers single-site superconductors. Thus, we can expect the exact coincidence only when the ABSs rarely mix with the bulk states: For $\phi \sim \pi$, where the ABSs are distinct from the bulk states, Eqs. (S36) and (S40) give

$$\begin{aligned} E_{2,3} &= \pm\sqrt{(t-\Delta)^2 + \frac{1}{4}t\Delta(\phi-\pi)^2}\,, \\ E_{\pm}^{\rm lit} &= \pm\sqrt{(1-T_N)\Delta_{\rm lit}^2 + \frac{1}{4}T_N\Delta_{\rm lit}^2(\phi-\pi)^2}\,, \end{aligned} \tag{S41}$$

and thus, they coincide exactly by the identification $(t-\Delta)^2 = (1-T_N)\Delta_{\rm lit}^2$ and $t\Delta \sim T_N\Delta_{\rm lit}^2$. In contrast, they show a deviation for $\phi \sim 0$, since the ABSs are much closer to the bulk states in this situation. See Fig.S2 (d-e).

*Comparison with model in Eq. (6)*

The ABSs in Eq. (S39) exhibit the exactly same $\phi$-dependence in Eq. (S40) with $T_{\rm N} = 1$ and $(\Delta\sqrt{2C}/A) = \Delta_{\rm lit}$.

## S4. ANALYTICAL EXPRESSIONS FOR THE SUPERCURRENTS OF THE EFFECTIVE MODELS

This section presents analytical expressions of the supercurrents associated with the ABSs of the effective models in Eqs. (3), and (5) of the main text. The ABSs for these models are given by Eqs. (4) and (6).

For the model in Eq.(3), the total supercurrent is given by the two occupied ABSs, namely, $E_{1,2}$, where $E_{1(2)}$ is the lower (higher) negative real energy ABS in Eq. (4) of the main text. From Eq. (2) of the main text, each of these ABSs carries the supercurrent of $I_{1(2)} = (e/\hbar)dE_{1(2)}/d\phi$, which is then given by

$$\begin{aligned} I_1(\phi) &= \frac{e}{\hbar}\frac{dE_1}{d\phi} = -\frac{t^2\Delta\sin(\phi)}{4\sqrt{t^2\sin^2(\phi/2)-\gamma^2}\sqrt{\delta^2-\gamma^2+2\Delta\sqrt{t^2\sin^2(\phi/2)-\gamma^2}}}\,, \\ I_2(\phi) &= \frac{e}{\hbar}\frac{dE_2}{d\phi} = \frac{t^2\Delta\sin(\phi)}{4\sqrt{t^2\sin^2(\phi/2)-\gamma^2}\sqrt{\delta^2-\gamma^2-2\Delta\sqrt{t^2\sin^2(\phi/2)-\gamma^2}}}\,, \end{aligned} \tag{S42}$$

where $\delta = t^2 + \Delta^2$ and $\gamma = (\Gamma_L - \Gamma_R)/2$. As discussed in the main text, EPs appear at finite real energies when $t^2\sin^2(\phi/2) = \gamma^2$, which then implies that both supercurrents diverge at EPs but with opposite sign. Thus, at EPs the divergent profile of the total supercurrent, the sum of Re$I_1$ and Re$I_1$, is suppressed, giving rise to a smooth behavior across EPs. Between EPs, when $t^2\sin^2(\phi/2) < \gamma^2$, the current exhibits both real and imaginary parts due to finite phase dependent real and imaginary ABSs, as seen in Fig. 2 of the main text.

For the second model in Eq.(5), we have two ABSs around zero energy. See Eq. (6) in the main text. Then, the occupied ABS contributes to the supercurrent, as in Eq. (2) of the main text. Thus, the total supercurrent in the second model is given by

$$I(\phi) = \frac{e}{\hbar}\frac{dE_-}{d\phi} = +\Delta t^4\frac{\sin(\phi)}{\sqrt{C+2t^4A\cos(\phi)}} \tag{S43}$$

where $C = 4t^4[2t^4+(2t^2-2\gamma^2+\Gamma^2)\Delta^2]+2[(t^2-\gamma^2)^2+\Gamma^2(\Gamma^2-2\gamma^2)]\Delta^4-\gamma^2\Delta^6$ and $A = 4t^4+\Delta^4+2\Delta^2\left(-\gamma^2+\Gamma^2+2t^2\right)$. Here, EPs form at zero-real energy when $C + 2t^4A\cos(\phi) = 0$, implying that the supercurrent diverges at these EPs. Unlike the supercurrent in the first model, no suppression occurs for Re$I$ because no other energy level contributes to the total supercurrent. Thus, EPs enhance the supercurrent, as we observe in Fig. 3(c) of the main text.

## S5. DERIVATION OF THE JOSEPHSON CURRENT FORMULA EQ. (2)

Here, we derive the semi-classical formula for the Josephson current in the junction coupled to an electron reservoir (metal), Eq. (2) of the main text. First, we note that the Josephson current is an equilibrium current that flows only

between superconductors with a phase difference; otherwise, it gives an unknown equilibrium current in a Hermitian system. We note that the original Hamiltonian for the Josephson junction and the coupled metal is Hermitian [Eq. (S1)], and we consider the equilibrium state. Therefore, the current cannot flow into the attached metal, and quasi-particles in the junction suffice to evaluate the Josephson current. We do not need to explicitly include quasi-particles in the metal, whatever is the coupling strength between the junction and the metal. Whereas a quasi-particle in the Josephson junction may have a complex spectrum due to the coupling to the metal, we can strictly include this effect by using the effective Hamiltonian $H_{\mathrm{eff}}(\phi)$. In other words, the effective Hamiltonian $H_{\mathrm{eff}}(\phi)$ in the junction well describes the current, which includes the influence of the metal implicitly as the non-Hermiticity of $H_{\mathrm{eff}}(\phi)$; This is a standard approach to account for normal leads in quantum transport even when multiple normal leads are coupled. See Ref. [3].

From the argument above, we can start with the Bogoliubov-de Gennes equation for quasi-particles in the junction

$$H_{\mathrm{eff}}(\phi)|E_n(\phi)\rangle = E_n(\phi)|E_n(\phi)\rangle, \tag{S44}$$

where $\phi = \phi_{\mathrm{R}} - \phi_{\mathrm{L}}$ is the phase difference between the right and left superconductors of the junction. Note that $E_n(\phi)$ is not necessarily real since $H_{\mathrm{eff}}(\phi)$ is non-Hermitian. Then, the time-evolution of a quasiparticle is given by

$$|\psi(t)\rangle = e^{-i(E_n(\phi)/2\hbar)t} U(\varphi)|E_n(\phi)\rangle, \tag{S45}$$

where $U(\varphi)$ with $\varphi = (\phi_{\mathrm{R}} + \phi_{\mathrm{L}})/2$ is a gauge degrees of freedom and the factor $1/2$ in the exponent originates from the redundancy in the Nambu space.

Using the semi-classical representation of the charge operators $Q_{\alpha=R,L}$ in the right and left superconductors in terms of their phases $\phi_{\mathrm{R}}$ and $\phi_{\mathrm{L}}$ in the pair potentials (or gap functions),

$$Q_\alpha = 2ei\frac{d}{d\phi_\alpha}\,, \tag{S46}$$

we have

$$Q_{\mathrm{R}} + Q_{\mathrm{L}} = 2ei\left.\frac{\partial}{\partial\varphi}\right|_{\phi}, \quad \frac{Q_{\mathrm{R}} - Q_{\mathrm{L}}}{2} = 2ei\left.\frac{\partial}{\partial\phi}\right|_{\varphi}. \tag{S47}$$

Thus, we can evaluate these charges of the quasi-particle at time $t$ as

$$\begin{aligned}\langle Q_{\mathrm{R}} + Q_{\mathrm{L}}\rangle_t &= \left(\frac{\langle\psi(t)|}{\|\langle\psi(t)|\|}\right) 2ei\frac{\partial}{\partial\varphi}\left(\frac{|\psi(t)\rangle}{\||\psi(t)\rangle\|}\right)\\ &= 2ei[U^\dagger(\varphi)\partial_\varphi U(\varphi)], \end{aligned}\tag{S48}$$

$$\begin{aligned}\langle (Q_{\mathrm{R}} - Q_{\mathrm{L}})/2\rangle_t &= \left(\frac{\langle\psi(t)|}{\|\langle\psi(t)|\|}\right) 2ei\frac{\partial}{\partial\phi}\left(\frac{|\psi(t)\rangle}{\||\psi(t)\rangle\|}\right)\\ &= \frac{e}{\hbar}\frac{d\mathrm{Re}E_n(\phi)}{d\phi}t + 2ei\langle E_n(\phi)\partial_\phi E_n(\phi)\rangle. \end{aligned}\tag{S49}$$

Note that we need to use the normalized state $|\psi(t)\rangle/\||\psi(t)\rangle\|$ for the evaluation to keep the Hermiticity of the charge operators. Here, we note that the total charge of the junction in Eq. (S48) does not change as a function of time $t$, which is consistent with our argument that the current does not flow into the metal.

Then, from Eq.(S49), we have the semi-classical formula for the current carried by the quasi-particle $|E_n(\phi)\rangle$ as

$$I_n(\phi) = \frac{d\langle (Q_{\mathrm{R}} - Q_{\mathrm{L}})/2\rangle}{dt} = \frac{e}{\hbar}\frac{d\mathrm{Re}E_n(\phi)}{d\phi}\,, \tag{S50}$$

where we have used the fact that the second term in Eq. (S49) is $t$-independent, so it does not contribute to the current. Among these quasi-particles, negative energy states occupy the ground state, contributing to the Josephson current. Thus, the total current is given by

$$I(\phi) = \frac{e}{\hbar}\sum_{\mathrm{Re}E_n(\phi)\leq 0}\frac{d\mathrm{Re}E_n(\phi)}{d\phi}\,, \tag{S51}$$

which coincides with the real part of Eq. (2) in the main text. Therefore, the real part of Eq. (2) gives the physical supercurrent as we argue in the main text.

Around the exceptional point at $\mathrm{Re}E_n(\phi) = 0$, $\mathrm{Re}E_n(\phi)$ behaves as $\mathrm{Re}E_n(\phi) = -\sqrt{s(\phi)}$ where $s(\phi)$ is a positive smooth function of $\phi$ that vanishes at the exceptional point. Thus, the intrinsic contribution of the exceptional point to the Josephson current diverges

$$I(\phi)|_{\mathrm{EP}} \sim -\frac{e}{2\hbar}\frac{s'(\phi)}{\sqrt{s(\phi)}}\bigg|_{s(\phi)\to 0} = \infty\,. \tag{S52}$$

Although the EP gives an intrinsic divergence in the Josephson current, as shown above, the imaginary part of the energy smears out the divergence since it obscures the band distinction. In particular, the band broadening mixes a negative energy state and its particle-hole partner state with a positive energy near EPs. Since an occupied state and its particle-hole partner contribute to the Josephson current with an opposite sign, the mixing suppresses the divergence in the Josephson current. Still, we can show that the EP enhances the Josephson current. To show the enhancement, let us consider an Andreev state near an EP,

$$E_n(\phi) = -\sqrt{s(\phi)} - i\Gamma\,, \tag{S53}$$

where $s(\phi)$ is given by

$$s(\phi) = a^2\cos^2(\phi/2) - b\gamma^2, \quad (a > 0,\, b \geq 0)\,. \tag{S54}$$

Here $a$ has the same dimension as $\gamma$, and $b \geq 0$ is dimensionless. At $\phi = \phi_0$ with $s(\phi_0) = 0$, $E_n(\phi)$ degenerates with the particle-hole partner $-E_n^*(\phi)$. For $b = 0$, the degeneracy is a simple level crossing, while for $b > 0$, the degeneracy is an exceptional point with a branch cut of square root. Because the mixing becomes significant when $|\mathrm{Re}E_n(\phi)|$ is comparable with the imaginary part $|\mathrm{Im}E_n(\phi)| = \Gamma$, the current growth near the exceptional point terminates at $\phi_1$ satisfying $\sqrt{s(\phi_1)} = \Gamma$. Thus, for $\gamma, \Gamma \ll a$, we can roughly estimate the maximal current as

$$I(\phi)|_{\max} \sim \frac{e}{\hbar}\frac{d\mathrm{Re}E_n(\phi)}{d\phi}\bigg|_{\phi=\phi_1} = \frac{e}{\hbar}\frac{a}{2}\sqrt{1 + b(\gamma/\Gamma)^2}\,, \tag{S55}$$

where we have used the relation

$$\phi_1 = \pi - \frac{2\Gamma}{a}\sqrt{1 + b(\gamma/\Gamma)^2}\,. \tag{S56}$$

We compare this estimation with the current without the EP. Since we can obtain the latter current by setting $b = 0$ in Eq.(S55), we conclude that the EP enhances the Josephson current by $\sqrt{1 + b(\gamma/\Gamma)^2}$. The enhancement factor is always larger than one when $b > 0$ so that an EP appears. The impact of the imaginary part of the energy (via $\Gamma$ and $\gamma$) on the supercurrent discussed here [Eqs. (S55)] is discussed in the Section on "Impact of the imaginary energy on the supercurrent" of the main text.

## S6. COMPARING THE SUPERCURRENT FORMULAS USED IN NON-HERMITIAN JOSEPHSON JUNCTIONS: ENHANCED SUPERCURRENT BY EXCEPTIONAL POINTS

Recently, Shen and collaborators in Ref. [10] derived a formula for the supercurrent in a non-Hermitian Josephson junctions given by

$$I(\phi) = -\frac{e}{\hbar\pi}\frac{d}{d\phi}\mathrm{Im}\mathrm{Tr}(H_{\mathrm{eff}}(\phi)\ln H_{\mathrm{eff}}(\phi))\,, \tag{S57}$$

where $H_{\mathrm{eff}}(\phi)$ is the effective Bogoliubov-de Gennes Hamiltonian defined by the retarded Green's function of the junction

$$G^r(\omega) = \frac{1}{\omega - H_{\mathrm{eff}}(\phi)}\,, \tag{S58}$$

and $\phi$ is the phase difference between the left and right superconductors of the junction. Below, we compare this formula [Eq. (S57)] with the semi-classical current formula used in the main text [Eq. (2)],

$$I_0(\phi) = \frac{e}{\hbar}\sum_{n\leq 0}\left[\frac{d\mathrm{Re}E_n(\phi)}{d\phi}\right]\,, \tag{S59}$$

where $E_n(\phi)$ represents the eigenvalues of $H_{\text{eff}}(\phi)$ and we take the summation $n$ for all $E_n(\phi)$s' with $\text{Re}E_n(\phi) \geq 0$. In particular, we show that both formulas support the idea that an exceptional point intrinsically has a divergent contribution to the Josephson current.

For this purpose, we first rewrite the formula in Eq. (S57) in terms of the eigenvalues $E_n(\phi)$ of $H_{\text{eff}}$. Using a unitary transformation, $H_{\text{eff}}$ can be an upper triangular form, of which the diagonal components are eigenvalues of $H_{\text{eff}}$. Thus, Eq. (S57) is recast into

$$I(\phi) = -\frac{e}{\hbar\pi}\frac{d}{d\phi}\text{Im}\left(\sum_n E_n(\phi)\ln E_n(\phi)\right), \tag{S60}$$

where we take the summation $n$ for all possible eigenvalues $E_n(\phi)$. Since $H_{\text{eff}}(\phi)$ has the following particle-hole symmetry,

$$CH^*_{\text{eff}}(\phi)C^\dagger = -H_{\text{eff}}(\phi), \tag{S61}$$

with a unitary matrix $C$, an eigenvalue $E_n$ forms a pair with another eigenvalue $-E_n^*$. Therefore, we can further rewrite the above equation as

$$\begin{aligned} I(\phi) &= -\frac{e}{\hbar\pi}\frac{d}{d\phi}\text{Im}\sum_{n\leq 0}\left(E_n(\phi)\ln E_n(\phi) - E_n^*(\phi)\ln(-E_n^*(\phi))\right) \\ &= -\frac{e}{\hbar\pi}\frac{d}{d\phi}\text{Im}\sum_{n\leq 0}\big(\text{Re}E_n(\phi)\ln(-E_n(\phi)/E_n^*(\phi)) + i\text{Im}E_n(\phi)\ln\big(-|E_n(\phi)|^2\big)\big) \\ &= -\frac{e}{\hbar\pi}\frac{d}{d\phi}\sum_{n\leq 0}\big(\text{Re}E_n(\phi)\text{Im}[\ln(-E_n(\phi)/E_n^*(\phi))] + \text{Im}E_n(\phi)\ln|E_n(\phi)|^2\big), \end{aligned} \tag{S62}$$

where now we perform the summation $n$ for all $E_n$s' with $\text{Re}E_n(\phi) \leq 0$. Then, using the relation,

$$\ln(-E_n(\phi)/E_n^*(\phi)) = 2i\arctan(-\text{Re}E_n(\phi)/\text{Im}E_n(\phi)), \tag{S63}$$

we have

$$I(\phi) = -\frac{e}{\hbar\pi}\frac{d}{d\phi}\sum_{n\leq 0}\left(2\text{Re}E_n(\phi)\arctan\left(\frac{-\text{Re}E_n(\phi)}{\text{Im}E_n(\phi)}\right) + \text{Im}E_n(\phi)\ln|E_n(\phi)|^2\right). \tag{S64}$$

To examine the influence of an EP on the Josephson current $I(\phi)$, let us consider an eigenenergy $E_0(\phi)$ given by

$$E_0 = -\sqrt{s(\phi)} - i\Gamma, \tag{S65}$$

where $s(\phi)$ is a real function of $\phi$. When $s(\phi) = 0$, $E_0(\phi)$ and $-E_n^*(\phi)$ are degenerate and form an EP at zero real energy, as we shown in Fig. 3(a) of the main text. Then, for $s(\phi) \geq 0$, $E_0$ contributes to the supercurrent [Eq. (S64)] as [11, 12]

$$\begin{aligned} I(\phi)|_{E_0} &= -\frac{e}{\hbar}\left[\frac{d\sqrt{s(\phi)}}{d\phi}\right]\left[\frac{2}{\pi}\arctan\left(\frac{\sqrt{s(\phi)}}{\Gamma}\right)\right] \\ &= I_0(\phi)|_{E_0}\left[\frac{2}{\pi}\arctan\left(\frac{\sqrt{s(\phi)}}{\Gamma}\right)\right], \end{aligned} \tag{S66}$$

where $I_0(\phi)|_{E_0}$ is the contribution of $E_0$ to the semi-classical current $I_0(\phi) = (-e/\hbar)[d\sqrt{s(\phi)}/d\phi]$. In the derivation of Eq. (S66), we have used the relation

$$2\frac{d}{d\phi}\arctan\left(\frac{\sqrt{s(\phi)}}{\Gamma}\right) = \Gamma\frac{d}{d\phi}\ln\big(s(\phi)+\Gamma^2\big) = \frac{2\Gamma}{s^2(\phi)+\Gamma^2}\frac{d\sqrt{s(\phi)}}{d\phi}. \tag{S67}$$

Now, we argue that there exists an intrinsic contribution of the EP to the Josephson current. Since $\Gamma$ is not related to the existence of the EP, we should take $\Gamma = 0$ to reveal the intrinsic contribution. Then, we find from Eq. (S66) that the Josephson current coincides with the semi-classical formula

$$I(\phi)|_{E_0} = I_0(\phi)|_{E_0}, \tag{S68}$$

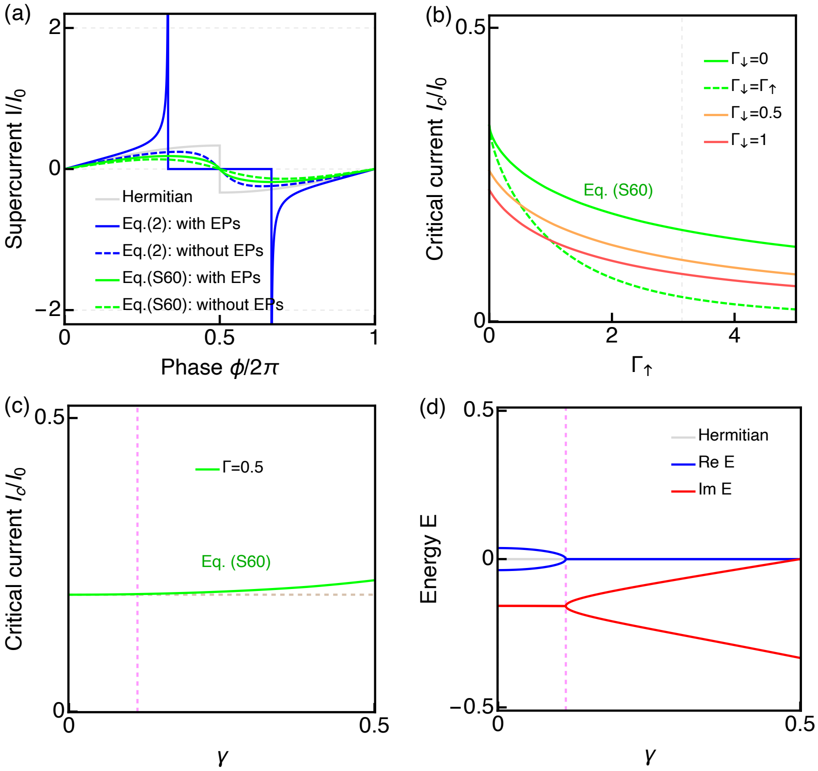


FIG. S3. (a) Supercurrent as a function of the phase difference for the model given by Eq. (5) of the main text. The blue and green solid curves are obtained using Eqs. (2) in the main text and Eq. (S60), respectively, in both cases with $\Gamma_\uparrow = 2$ and $\Gamma_\downarrow = 0$ ensuring the formation of EPs. The respective dashed curves correspond to $\Gamma_\uparrow = 1$ and $\Gamma_\downarrow = 1$ without EPs, while the gray curve depicts the Hermitian regime. (b) Critical current as a function of $\Gamma_\uparrow$ and distinct values of $\Gamma_\downarrow$. (c) Critical current as a function of $\gamma = (\Gamma_\uparrow - \Gamma_\downarrow)/2$ at fixed $\Gamma = (\Gamma_\uparrow + \Gamma_\downarrow)/2 = 0.5$. In (b,c), the horizontal gray line marks the value of the critical current in the Hermitian regime; in (c) the horizontal brown dashed line marks the critical current without EPs at $\gamma = 0$. (d) Real and Imaginary parts of the energy levels as a function of $\gamma$ for $\phi = \pi$ and $\Gamma = 0.5$. Vertical magenta dashed lines in (c,d) mark the beginning of the EP formation. Parameters: $\Delta = 1$, $t = 1$, $\varepsilon_\alpha = 0$.

which diverges at the EP. Thus, the intrinsic contribution of the EP to the Josephson current is divergent.

In actual experimental situations, we usually have a nonzero $\Gamma$. Since the arctangent factor in Eq.(S66) gives a cut-off, it obscures the divergent current due to the EP [13]. Still, as discussed in Sec. S5, the EP enhances the Josephson current for small $\Gamma$. From Eq.(S66), for $s(\phi)$ in Eq. (S54) with $\gamma, \Gamma \ll a$, we estimate the maximum of the Josephson current as

$$I(\phi)|_{\max} = \frac{e}{\hbar}\frac{d\mathrm{Re}E_n(\phi)}{d\phi}\left[\frac{2}{\pi}\arctan\left(\frac{\sqrt{s(\phi)}}{\Gamma}\right)\right]\Bigg|_{\phi=\phi_1} = \frac{e}{\hbar}\frac{a}{2}\sqrt{1+b(\gamma/\Gamma)^2}\left[\frac{2}{\pi}\arctan(1)\right]. \tag{S69}$$

Note that this estimation coincides with Eq. (S55) except for an $O(1)$ factor. Since we can obtain the current without the EP by putting $b = 0$ in Eq. (S69), we conclude again that the EP enhances the Josephson current by a factor of $\sqrt{1+b(\gamma/\Gamma)^2}$. The enhancement factor is always larger than one when $b > 0$ so that an EP appears. We confirm this enhancement numerically in the next section.

## S7. COMPARING THE BEHAVIOUR OF SUPERCURRENTS USING EQ. (2) AND EQ. (S60)

In this section, we compare the supercurrent in Eq. (2) of the main text with that in Eq. (S60). For this purpose, we consider the model described by Eq. (5) of the main text and also that on the realistic non-Hermitian SNS Josephson junction discussed in the last section of the main text entitled "NH JJs in superconductor-semiconductor hybrids."

For the model described by Eq. (5), we present the supercurrent as a function of the phase difference $\phi$ in Fig. S3(a), where the blue and green curves depict the currents in Eq. (2) and Eq. (S60), respectively. As we argued in the main

text, the current in Eq. (2) exhibits divergences at exceptional points (EPs) (blue solid curve), in contrast to that in the absence of EPs but still in the non-Hermitian (NH) regime (dashed blue curve). Whereas the current in Eq. (S60) does not show divergence at EPs, the current with EPs (green solid line) shows an enhancement in comparison with the case without EPs (green dashed line), in accordance with our argument in Eq.(S69). To further explore the enhancement, in Fig. S3(b) we plot the critical current (maximum supercurrent) as a function of $\Gamma_\uparrow$ for distinct values of $\Gamma_\downarrow$ using Eq. (S60). The critical current has larger values in the presence of EPs, which can be seen by comparing the solid and dashed green curves at $\Gamma_\downarrow = 0$. Further increasing $\Gamma_\downarrow$ reduces the overall profile of the current which happens due to the detrimental effect of the total dissipation $\Gamma = (\Gamma_\uparrow + \Gamma_\downarrow)/2$, but still, the critical currents (orange and red curves) for larger $\Gamma_\uparrow$ develop larger values than in the case without EPs (green dotted line). To shed more light on the enhancement of critical currents, in Fig. S3(c) we plot them as a function of non-Hermitian asymmetry $\gamma = (\Gamma_\uparrow - \Gamma_\downarrow)/2$ at fixed total non-Hermiticity $\Gamma = 0.5$. At very small $\gamma$, the current remains constant, but as $\gamma$ exceeds a critical value (purple dotted line), the current develops an enhancement with respect to $\gamma = 0$. Interestingly, the critical value of $\gamma$ at which the current enhancement starts corresponds to that promoting the formation of EPs; see Fig. S3(d). Thus, the current obtained by Eq. (S60) exhibits an enhancement due to EPs, which aligns with the idea discussed in the main text. We note that the currents in Eq.(S60) with non-Hermiticity are less than that in the Hermitian case. Still, this suppression stems from the band broadening due to the total dissipation $\Gamma = (\Gamma_\uparrow + \Gamma_\downarrow)/2$ and is nothing related to the presence or absence of EPs.

We now consider the non-Hermitian Rashba SNS junction. Figure S4(a) shows the real and imaginary parts of the spectra as a function of $\phi$, where non-Hermiticity is only in the N region, with $\Gamma_\uparrow = 3.5$meV and $\Gamma_\downarrow = 0$meV. This figure is the same as those in Fig. 4(c) of the main text, showing the phase-dependent imaginary part as well as the formation of EPs. Figure S4(c) shows the corresponding supercurrents as a function of $\phi$, where blue and green curves use the formulas in Eq. (2) of the main text and Eq. (S60), respectively. We observe that the supercurrent (blue solid curve or green solid curve) develops a divergent or enhanced profile at EPs, in line with what is discussed in the main text. To make the enhancement more evident, we compare the currents with those in junctions having a homogeneous non-Hermiticity all over the SNS junction with $\Gamma_\uparrow = 3.5$meV. As shown in Fig. S4(b), in this case, all the energy levels acquire the same constant imaginary part, and no EPs appear in the junction. The corresponding supercurrents (blue and green dotted curves) in Fig. S4(c) are much less than those in the junction with EPs (blue and green solid curves).

Interestingly, we also find that the supercurrent in Eq. (S60) may acquire larger values than its Hermitian counterpart depending on the profile of the imaginary energy. To realize such a situation, now consider a non-Hermitian Josephson junction with non-Hermiticity only at the outer ends of the S regions. Here EPs form for a strong non-Hermiticity as depicted in Fig. S4(d), and the imaginary part exhibits a distinct behavior as compared to Fig. S4(a). For comparison, we also consider the junction with a homogeneous non-Hermiticity all over the N and S regions. As shown in Fig. S4(e), the latter case does not exhibit EPs and the imaginary part is the same for all levels and does not disperse with $\phi$. Again, we observe that EPs enhance the Josephson current: The supercurrents with EPs (blue and green solid curves) are larger than those without EPs (blue and green dotted curves). Remarkably, in the present case, EPs enhance the supercurrent even more than in the Hermitian case (grey curve).

We emphasize that the enhanced supercurrent profile occurs around EPs, and, since the only difference between Figs. S4(a) (Figs. S4(d)) and Fig. S4(b) (Fig. S4(e)) is the emergence of EPs, the mechanism behind the enhancement must be the EPs. Because the regime presented in Fig. S4 corresponds to a finite topological Josephson junction, we have also studied a minimal model with four Majorana zero modes coupled to reservoirs and verified that all the presented findings hold, especially those related to the emergence of EPs and enhanced supercurrents at EPs [14]. Therefore, EPs enhance supercurrents non-Hermitian Josephson junctions.

---


[1] J. Cayao, E. Prada, P. San-Jose, and R. Aguado, SNS junctions in nanowires with spin-orbit coupling: Role of confinement and helicity on the subgap spectrum, Phys. Rev. B **91**, 024514 (2015).

[2] J. Cayao and A. M. Black-Schaffer, Exceptional odd-frequency pairing in non-hermitian superconducting systems, Phys. Rev. B **105**, 094502 (2022).

[3] S. Datta, *Electronic transport in mesoscopic systems* (Cambridge university press, 1997).

[4] S. De Franceschi, L. Kouwenhoven, C. Schönenberger, and W. Wernsdorfer, Hybrid superconductor–quantum dot devices, Nat. Nanotech. **5**, 703 (2010).

[5] K. Kawabata, K. Shiozaki, M. Ueda, and M. Sato, Symmetry and topology in non-Hermitian physics, Phys. Rev. X **9**, 041015 (2019).

[6] K. Kawabata, T. Bessho, and M. Sato, Classification of exceptional points and non-Hermitian topological semimetals,

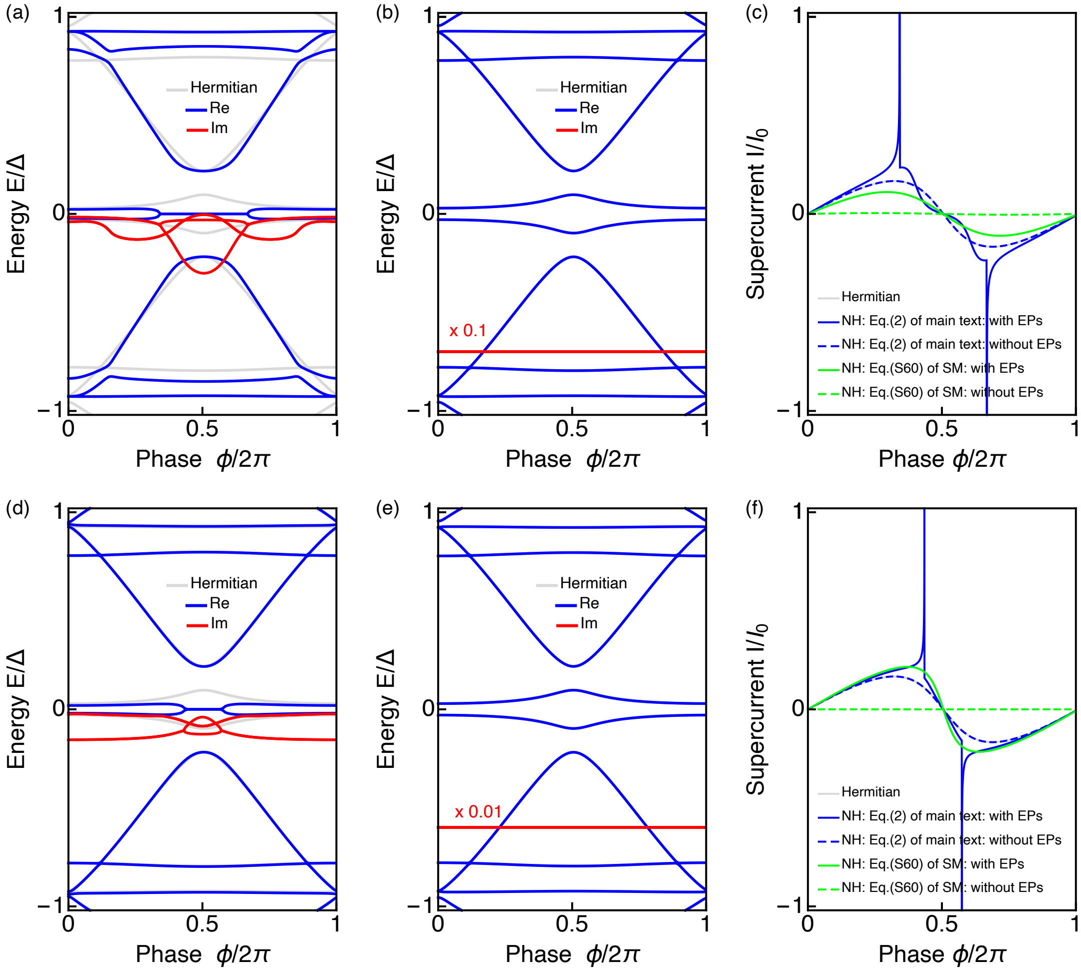


FIG. S4. (a) Phase dependent spectrum for a non-Hermitian SNS Josephson junction with non-Hermiticity in the middle N region $\Gamma_{\uparrow} = 3.5$meV and $\Gamma_{\downarrow} = 0$; EPs form in this regime. The blue (red) curves correspond to the real (imaginary) part of the spectrum, while the gray curves to the spectrum in the Hermitian regime. (b) Same as in (a) for an homogeneous non-Hermiticity all over the junction and equal to $\Gamma_{\sigma} = 3.5$meV; no EPs form in this regime. (c) Phase dependent supercurrents corresponding to the spectra in (a) using Eqs. (2) in the main text and Eq. (S60), indicated by solid blue and green curves. The respective dashed curves correspond to the supercurrents for the case without EPs in (b), while the gray curves is for the Hermitian regime. (d) The same as in (a) but with non-Hermiticity at the outer ends of the S regions given by $\Gamma_{\sigma} = 30\,$meV, while in (e) these couplings are homogeneous all over the junction. (f) The same as in (c) but for (d,e). Parameters: $\alpha = 40$meVnm, $\Delta = 0.5$meV, $\mu_{\rm N(S)} = 0.5$meV, $L_{\rm N} = 20$nm, $L_{\rm S} = 0.5\mu$m, $\Gamma_{\downarrow} = 0$, $I_0 = e\Delta/\hbar$

Phys. Rev. Lett. **123**, 066405 (2019).
[7] A. Furusaki and M. Tsukada, A unified theory of clean Josephson junctions, Physica B: Condensed Matter **165**, 967 (1990).
[8] C. Beenakker, Three “universal” mesoscopic Josephson effects, in *Transport phenomena in mesoscopic systems: Proceedings of the 14th Taniguchi symposium, Shima, Japan, November 10-14, 1991*, Vol. 109 (Springer-Verlag, 1992) p. 235.
[9] J. Sauls, Andreev bound states and their signatures, Philosophical Transactions of the Royal Society A: Mathematical, Physical and Engineering Sciences **376**, 20180140 (2018).
[10] P.-X. Shen, Z. Lu, J. L. Lado, and M. Trif, Non-hermitian persistent current transport, arXiv:2403.09569 (2024).
[11] C. W. J. Beenakker, Josephson effect in a junction coupled to an electron reservoir, arXiv:2404.13976 (2024).
[12] D. M. Pino, Y. Meir, and R. Aguado, Thermodynamics of non-Hermitian Josephson junctions with exceptional points, arXiv: 2405.02387 (2024).
[13] As discussed in Ref. [11], Γ introduces a phase decoherence. Thus, it suppresses the Josephson current.
[14] J. Cayao and M. Sato, to be published elsewhere.
